# Supplementary material for: Bias correction in treatment effect estimates following data-driven biomarker cutoff selection
Source: arXiv:2504.19776 source file (2025-04-28)
Supplement: Supplementary file 1 [file Bias_estimation_supplementary_figures_and_tables.pdf]

# Supplementary Figures and Tables

## Supplementary Figures

**Figure S1. Comparison of maximum likelihood estimation (MLE) in different subgroups across simulations**

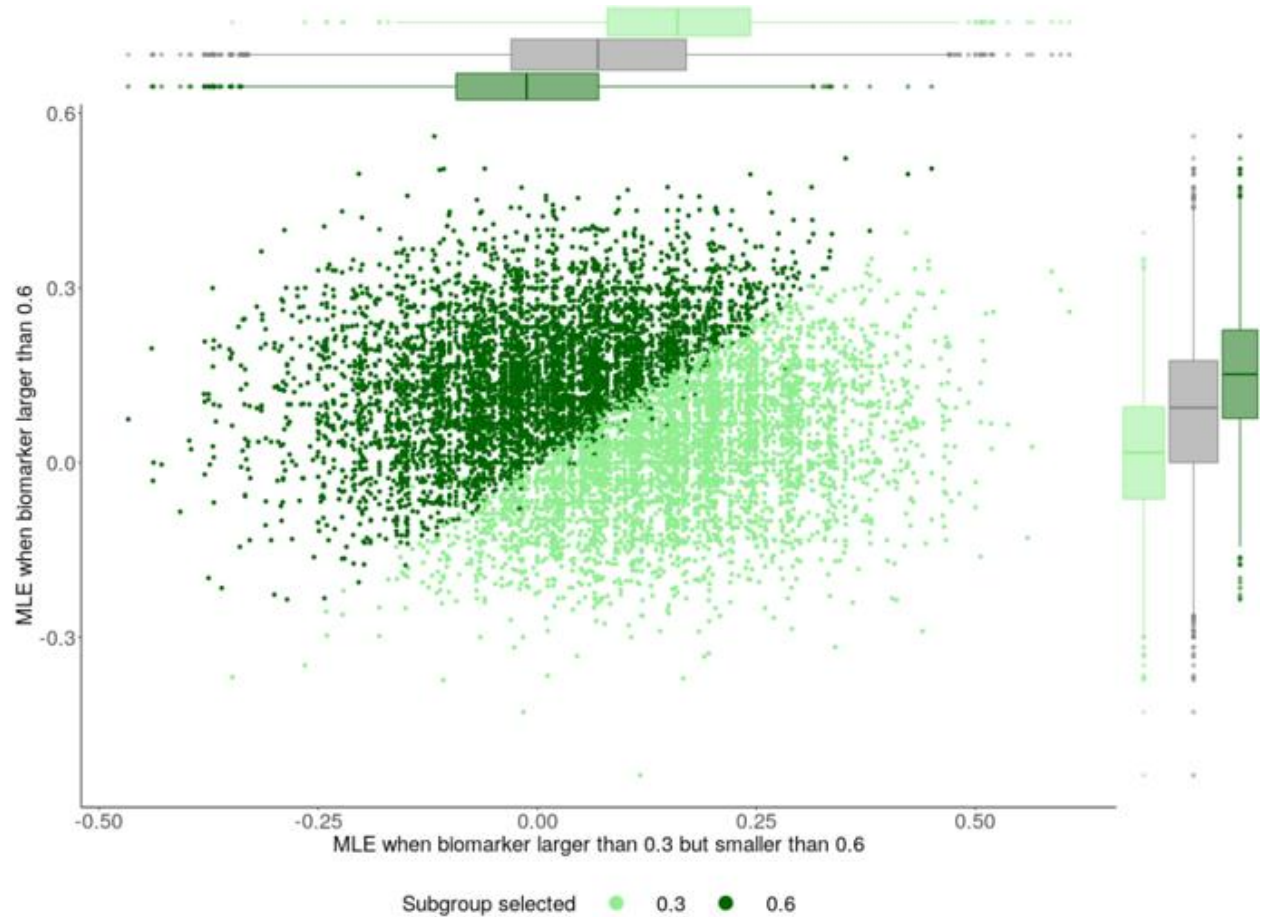

Each dot represents one simulation and there are 10,000 simulations conducted. The x-axis represents the MLEs for the subgroup whose biomarker value falls between 0.3 and 0.6 and the y-axis represents the MLEs for the subgroup whose biomarker value is larger than 0.6. Light green dots represent the simulations when cutoff 0.3 is selected and the dark green dots represent the cutoff value of 0.6, and the boxplots with corresponding color represent the distribution of MLEs on the simulation with certain cutoff is selected. The grey boxplots represent the distribution of MLEs on all the simulation.

**Figure S2. Conditional bias under the first selection rule with five candidate cutoffs and 40 subjects per arm.**

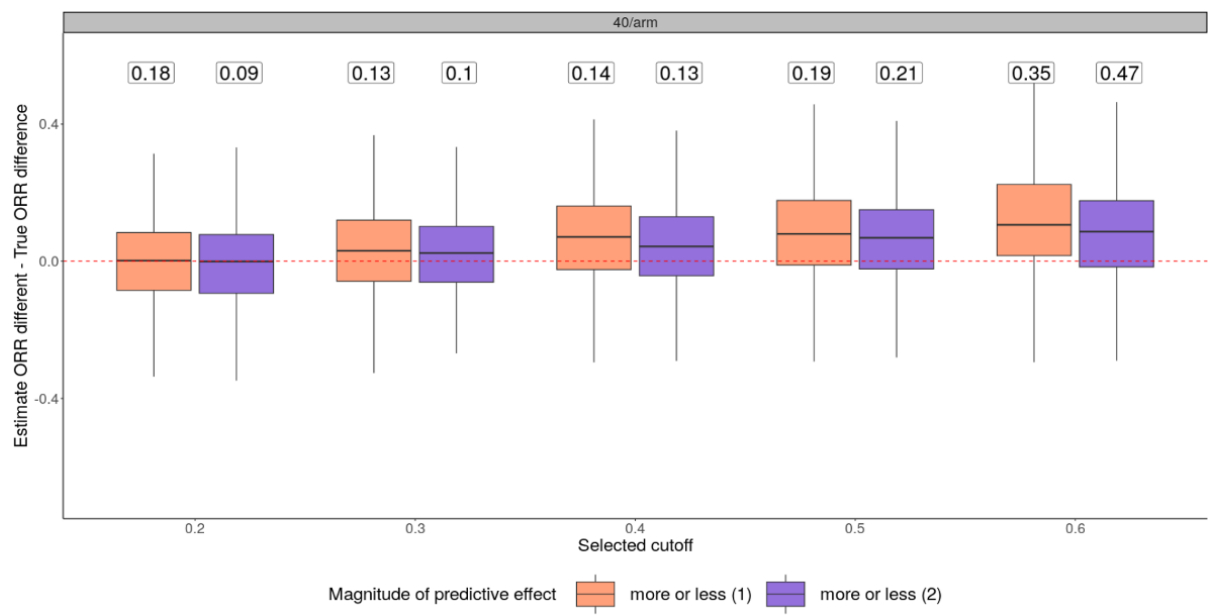

The x-axis represents the cutoff selected and the y-axis shows the conditional bias (estimated ORR difference - True ORR difference given selected cutoff). The numbers above each boxplot are the probabilities of each cutoff selected. The dashed line represents zero. Different color boxes represent different magnitudes of effect on predictive biomarkers.

**Figure S3. Conditional bias under the first selection rule with two or five candidate cutoffs and 40 subjects per arm.**

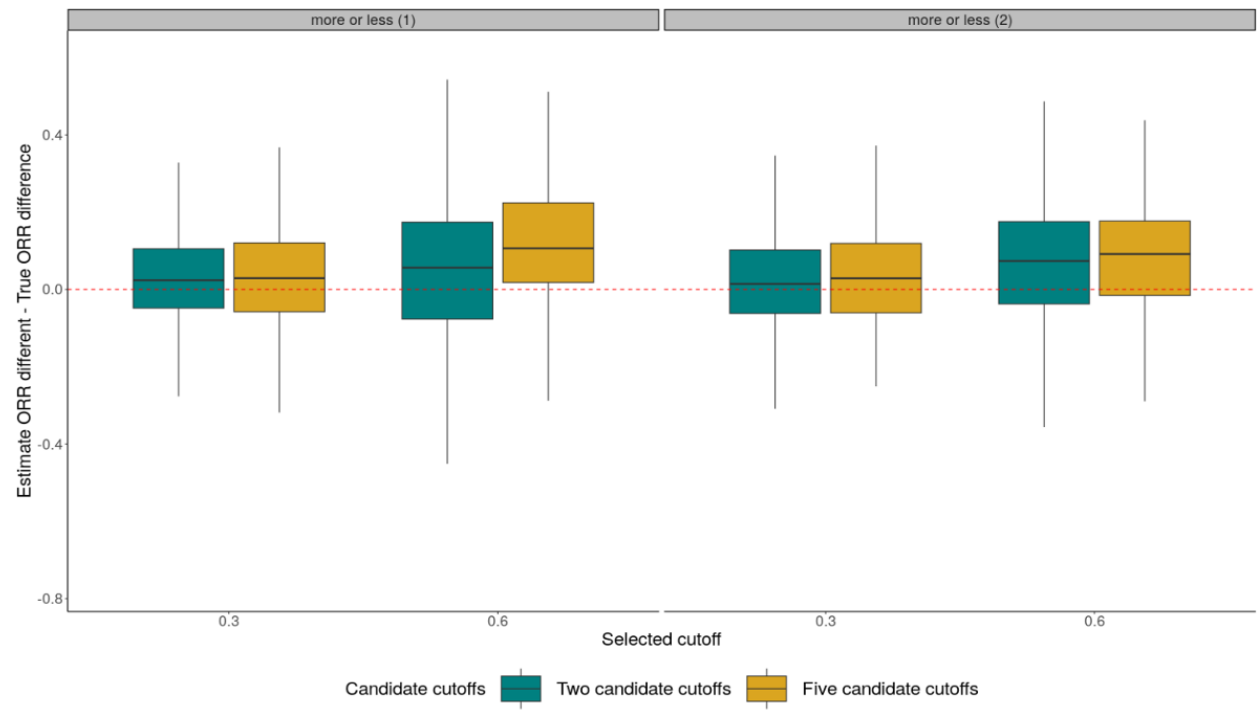

The x-axis represents the cutoff selected and the y-axis shows the conditional bias (estimated ORR difference - True ORR difference given selected cutoff). The dashed line represents zero. Different color boxes represent different numbers of candidate cutoffs.

**Figure S4. The probability of subgroup selection in different scenarios**

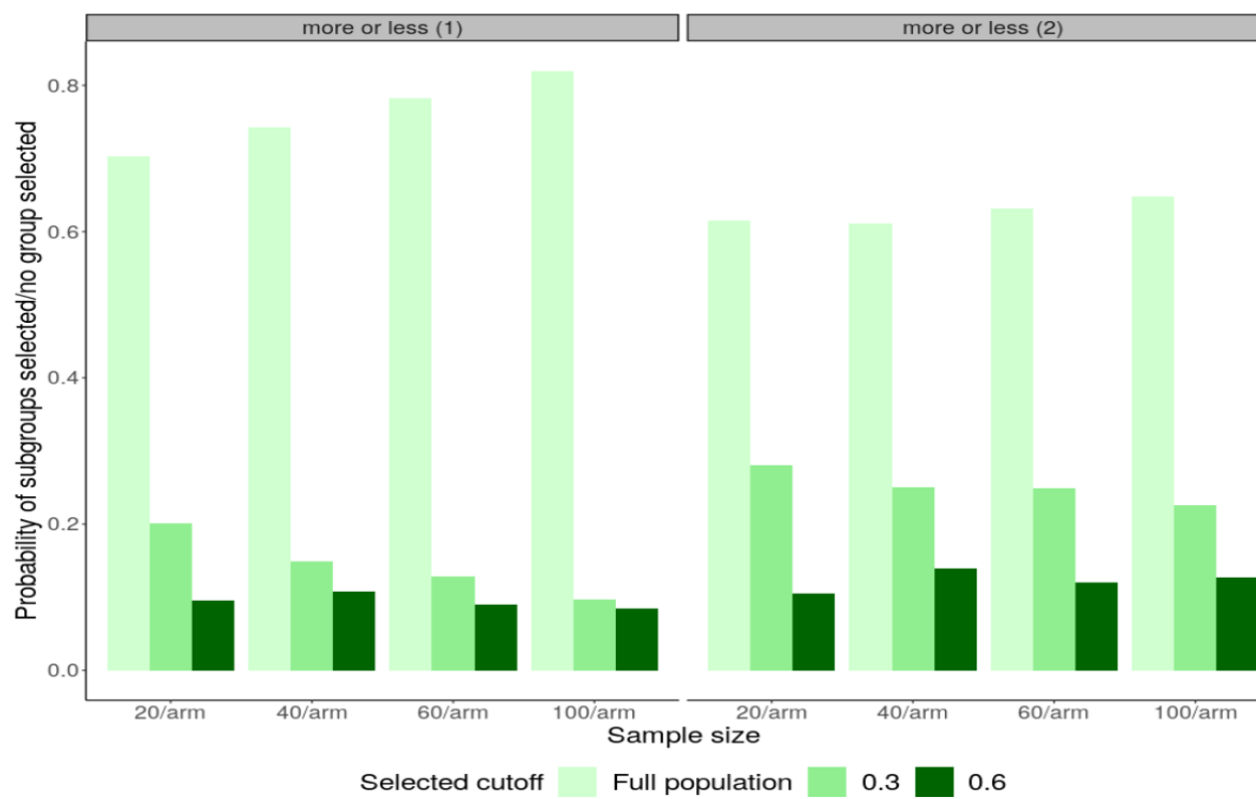

The x-axis is different sample sizes, and the y-axis is the probability of subgroup or no group selection. Each color bar stands for different subgroups, or the full population selected.

**Figure S5. Conditional bias under the second selection rule with two or five candidate cutoffs and 40 subjects per arm.**

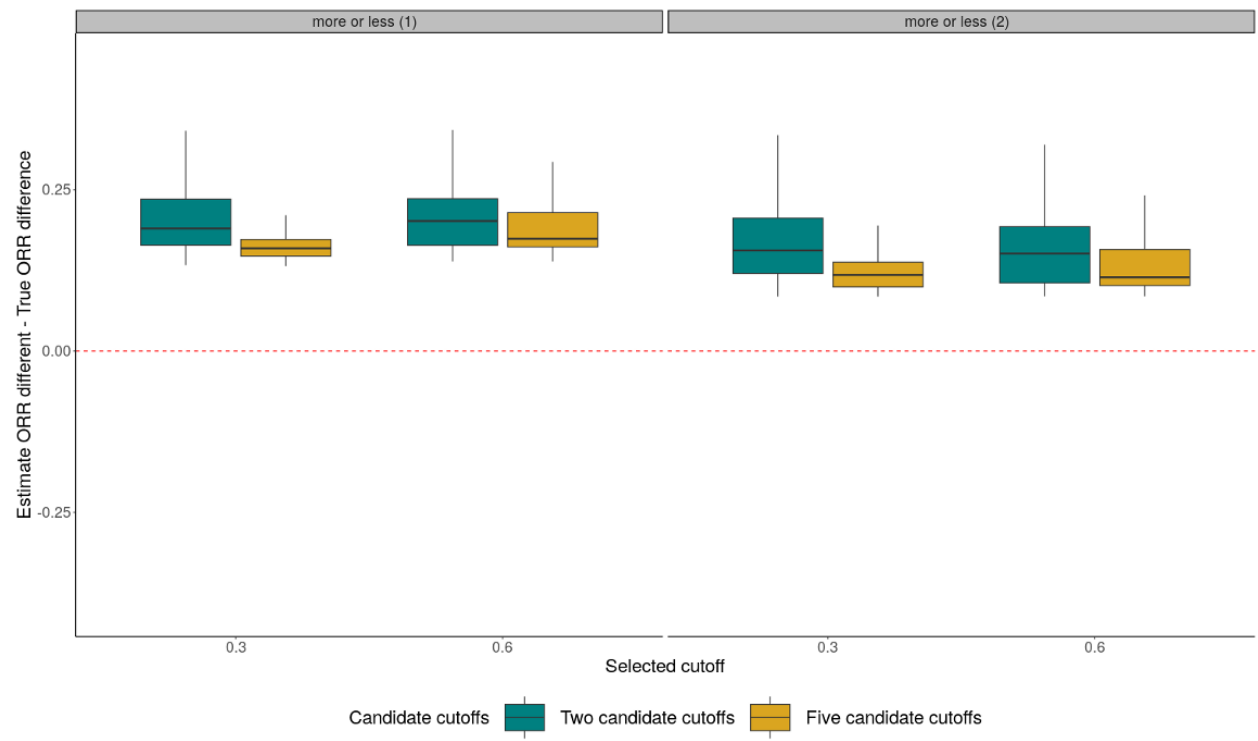

The x-axis represents the cutoff selected and the y-axis shows the conditional bias (estimated ORR difference - True ORR difference given selected cutoff). The dashed line represents zero. Different color boxes stand for different numbers of candidate cutoffs.

**Figure S6. Conditional bias for Bootstrap bias correction and MLE under the second selection rule with two candidate cutoffs when cutoff 0.6 is selected.**

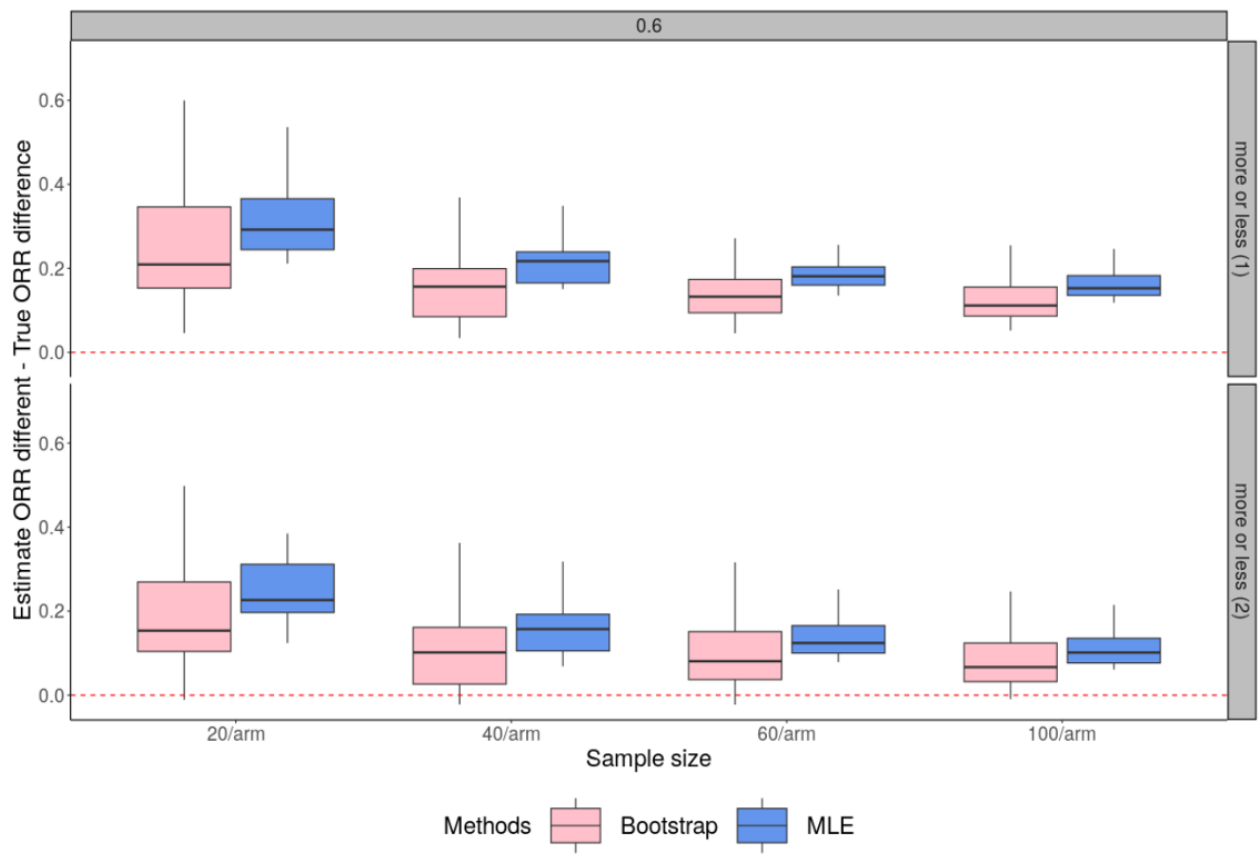

The x-axis is the sample size, and the y-axis shows the conditional bias (Estimated ORR difference - True ORR difference given selected cutoff). The first row is the conditional bias when more or less (1) model is used, and the second row is for more or less (2) model. The dashed line stands for zero. Different color boxes stand for different methods.

**Figure S7. Conditional bias for Bootstrap bias correction and MLE under the second selection rule with two candidate cutoffs when cutoff 0.3 is selected.**

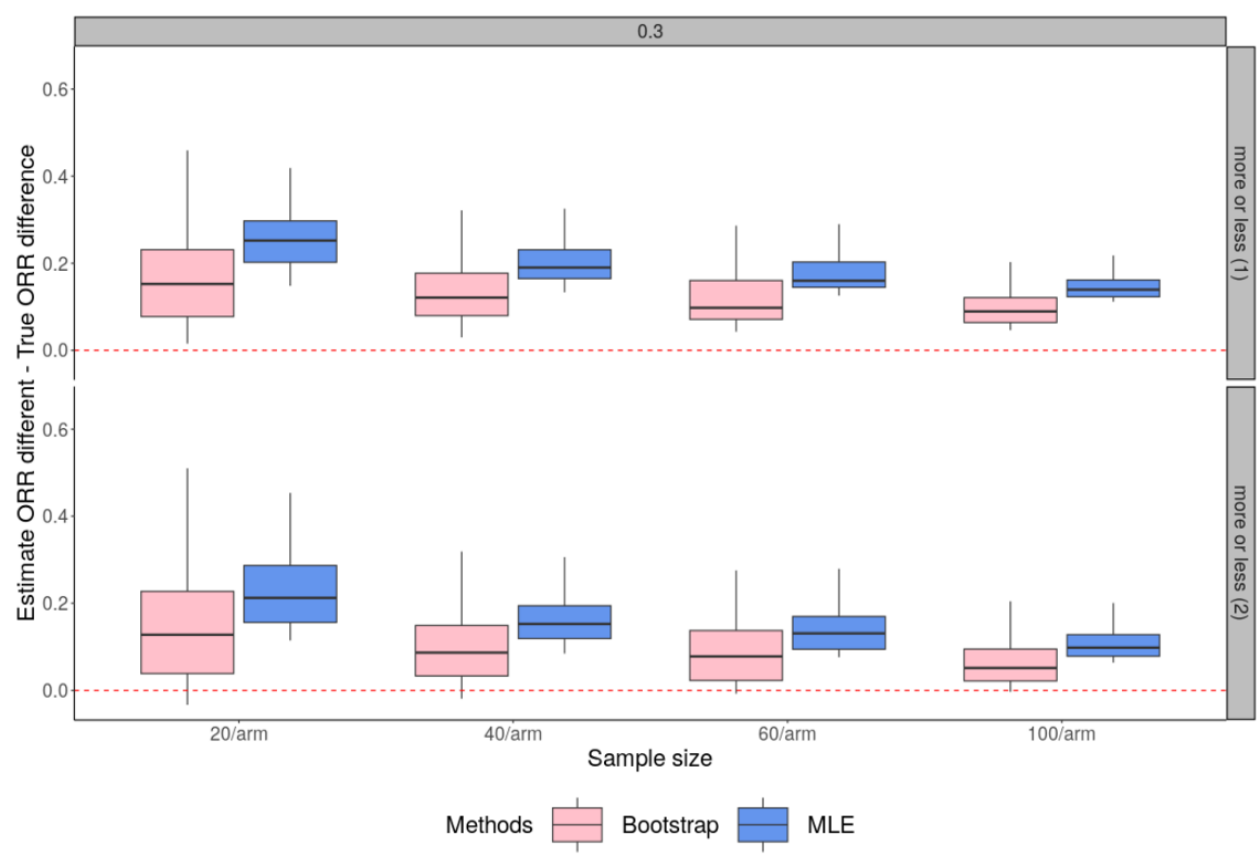

The x-axis is the sample size, and the y-axis shows the conditional bias (Estimated ORR difference - True ORR difference given selected cutoff). The first row is the conditional bias when more or less (1) model is used, and the second row is for more or less (2) model. The dashed line stands for zero. Different color boxes stand for different methods.

**Figure S8. Conditional bias for ABC with different priors and MLE under both selection rules with two candidate cutoffs**

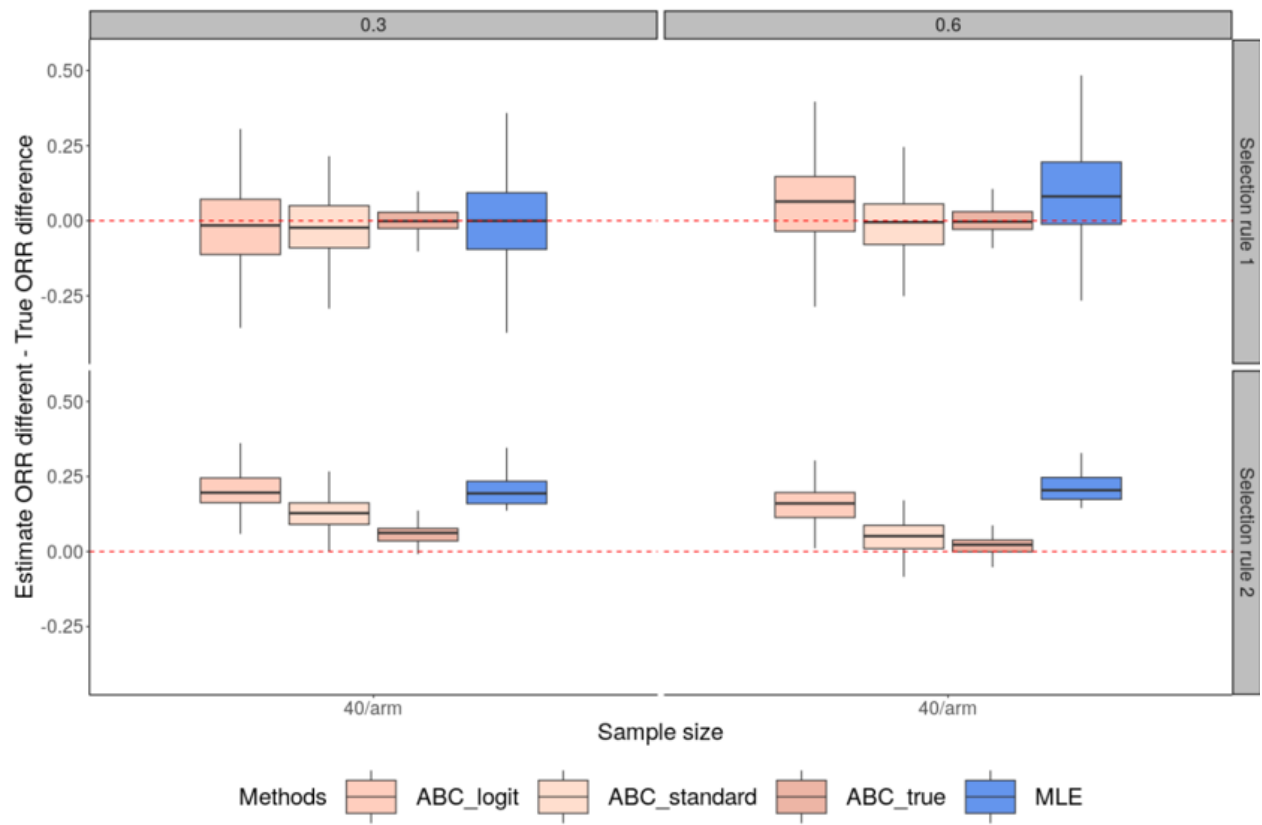

The x-axis is the sample size, and the y-axis shows the conditional bias (Estimated ORR difference - True ORR difference given selected cutoff). The first row is the conditional bias under the first selection rule, and the second row is under the second selection. The dashed line stands for zero. Different color boxes stand for different methods. "ABC\_logit" stands for the ABC method with priors using the estimated parameters as the mean value of normal distribution; "ABC\_standard" stands for the ABC method using standard normal distributions as priors; "ABC\_true" represents the ABC method with priors as the normal distributions using the true parameters as the mean value.

**Figure S9. Conditional bias for ABC with standard normal distributions as priors and MLE under both selection rules with two candidate cutoffs**

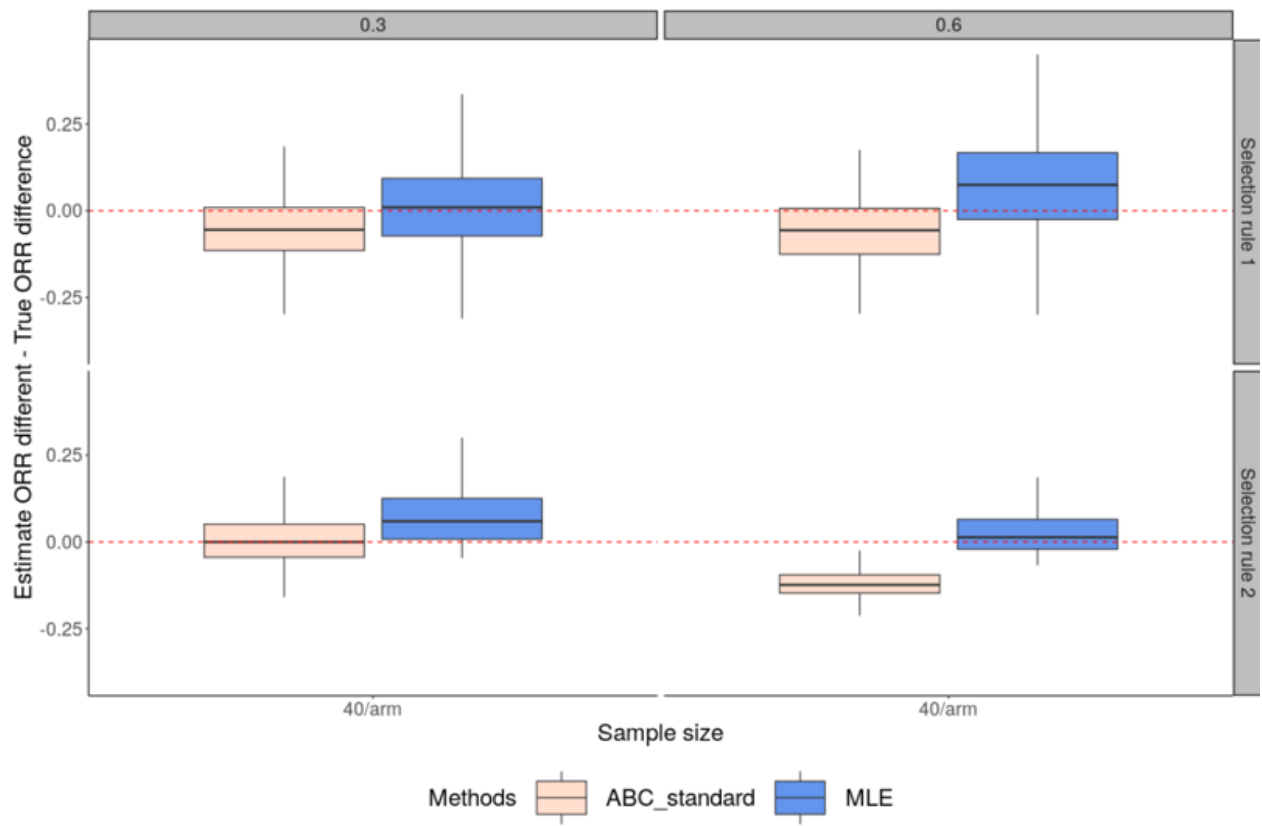

The x-axis is the sample size, and the y-axis shows the conditional bias (Estimated ORR difference - True ORR difference given selected cutoff). The first row is the conditional bias under the first selection rule, and the second row is under the second selection. The dashed line stands for zero. Different color boxes stand for different methods. "ABC\_standard" stands for the ABC method using standard normal distributions as priors.

**Table S1. Summary of Symbols, Parameters, and Their Descriptions**

| Symbol/parameter                          | Description                                                                        |
|-------------------------------------------|------------------------------------------------------------------------------------|
| $p_i$                                     | The conditional probability of observing an event for subject i.                   |
| $y_i$                                     | Observed response for subject i.                                                   |
| $x_i$                                     | Value of a continuous biomarker for subject i.                                     |
| $m_i$                                     | Treatment group where subject i is assigned; 1 = treatment E, 0 = control C        |
| $n$                                       | Total sample size.                                                                 |
| $n_{kER}$                                 | The number of subjects assigned to treatment in the subset k with response (ER).   |
| $n_{kEN}$                                 | The number of subjects assigned to treatment in the subset k without response(EN). |
| $n_{kCR}$                                 | The number of subjects assigned to control in the subset k with response (CR).     |
| $n_{kCN}$                                 | The number of subjects assigned to control in the subset k without response (CN).  |
| $p_{kE}, p_{kC}$                          | The ORRs in subset k for experimental treatment and control group.                 |
| $c_k$                                     | Cut-off values, $k=1, \dots, K$                                                    |
| $s_k$                                     | Subsets with biomarker value larger than $c_k$ , $s_k = \{i   x_i > c_k\}$         |
| $\theta_k, \hat{\theta}_k$                | True treatment effect in subset k and the general estimator of it.                 |
| $\theta_{select}, \hat{\theta}_{select}$  | True treatment effect in the selected subset and the general estimator of it.      |
| $\theta_{select,j}$                       | True treatment effect in the selected subset for simulation j.                     |
| $\hat{\theta}_{kMLE}$                     | MLE in subset k.                                                                   |
| $\hat{\theta}_{selectMLE}$                | MLE in the selected subset.                                                        |
| $\hat{\theta}_{selectMLE,j}$              | MLE in the selected subset for simulation j.                                       |
| $\hat{\theta}_{kABC}$                     | ABC-adjusted estimate in subset k.                                                 |
| $\hat{\theta}_{selectABC}$                | ABC-adjusted estimate in the selected subset.                                      |
| $\hat{\theta}_{selectABC,j}$              | ABC-adjusted estimate in the selected subset for simulation j.                     |
| $\hat{\theta}_{kBootstrap}$               | Bootstrap-adjusted estimate in subset k.                                           |
| $\hat{\theta}_{selectBootstrap}$          | Bootstrap-adjusted estimate in the selected subset.                                |
| $\hat{\theta}_{selectBootstrap,j}$        | Bootstrap-adjusted estimate in the selected subset for simulation j.               |
| $\Delta_{MLE s_k \text{ selected}}$       | Conditional bias of MLE given subset k selected.                                   |
| $\Delta_{ABC s_k \text{ selected}}$       | Conditional bias of ABC-adjusted estimate given subset k selected.                 |
| $\Delta_{Bootstrap s_k \text{ selected}}$ | Conditional bias of Bootstrap-adjusted estimate given subset k selected.           |
| $N$                                       | Number of simulations in each simulation setting.                                  |
| $N_k$                                     | Number of simulations where subset $s_k$ is selected.                              |
| $N_{simABC}$                              | Number of ABC simulation in each simulation.                                       |

**Table S2. The response rates for treatment or control in various subgroups and the full population.**

|  |                  |                  |
|--|------------------|------------------|
|  | More or less (1) | More or less (2) |
|--|------------------|------------------|

|                                                                                 |       |       |
|---------------------------------------------------------------------------------|-------|-------|
| The Response rate of control for all subgroups and the full population          | 0.400 | 0.400 |
| The response rate of treatment for the full population                          | 0.475 | 0.512 |
| The response rate of treatment for the subgroup with biomarkers larger than 0.3 | 0.483 | 0.531 |
| The response rate of treatment for the subgroup with biomarkers larger than 0.6 | 0.490 | 0.550 |
